# Supplementary material for: Context-aware Tree-based Deep Model for Recommender Systems
Source: arXiv:2109.10602 source file (2021-09-22)
Supplement: Supplementary file 1 [file supplement.tex]

%\section{Supplement}

%This material has 2 parts in total. Part A gives the additional experiment results to show the effectiveness of the multipath Tree. Part B gives the detailed derivation that confirms the efficiency of the Simplified parent fusion layer along with the increased quota setting.
\section{Data Preprocessing and Hyper-parameters}\label{appendix:hyper-param}

In this section, we give detailed configuration for the conducted experiments.

\textbf{\textit{Item-CF}}. We tune several most important hyper-parameters based on the testing set, i.e., the number of neighbours in Item-CF. 

\textbf{\textit{Data Preprocessing}}. We use the same user behavior feature as input. Each user behavior sequence has at most 69 user-item pairs. According to the timestamp, user behaviors are divided into 10 time windows. The ultimate user feature is the concatenation of each time window’s averaged item embedding vector of length 24.

\textbf{\textit{Sampling Strategy}}. This part is done during training. According to the scale of the datasets, we can easily infer that there are 22 and 23 levels of nodes starting from root (the $0^{th}$ level) for Amazon Books and UserBehavior respectively. We pick up both positive and negative samples from the $7^{th}$ level to leaf level. The positive samples from user behavior sequence can be easily mounted to nodes located in the leaf level and their ancestors of each upper level correspond to the positive samples of that level. Denote the ratio of positive and negative samples as $1:x$. The $x$ of for each level is listed as $\{0,1,2,3,4,5,6,7,8,9,10,11,12,13,14,15,17,19,22,$ $30,55,100\}$ for Amazon Books and $\{0,1,2,3,4,5,6,$ $7,8,9,10,11,$ $12,13,14,15,17$ $,19,22,25,30,76,200\}$ for UserBehavior.

\textbf{\textit{Graph Construction}}. In brief, we build the graph using the co-occurrence of nodes for each level of the tree index. Detailed process of graph building is shown in Algorithm \ref{alg:BuildGraph}.
\begin{algorithm}[]
\caption{Building Level-wise Graph for Tree}\label{alg:BuildGraph}
\begin{algorithmic}[2]
    \REQUIRE Initial binary tree $\mathcal{T}_b$, user behavior sequences of training data $behav_{i=1}^M$, $start\_sample\_level$
    \STATE Get $max\_level$ of $\mathcal{T}_b$
    \STATE $\mathcal{G} \gets \emptyset$
	\FOR {$l=max\_level, \dots, start\_sample\_level$}
		\FOR {$i=1, 2, \dots, M$}
			\STATE $seq_i \gets$ Trace each item in $behav_i$ up to the $level _l$ of $\mathcal{T}_b$.
			\IF{$u$ and $v$ appear together in $seq_i$ \textbf{and} the time interval between them $\leq 30$ minutes}
		    	\STATE Increase the weight of undirected edge $(u, v)$ by 1.
		    \ENDIF
		\ENDFOR
		\FOR {each node $u$ in $level_l$}
			\STATE $\{v\}_{i=1}^K \gets$ Pick the other endpoint of all undirected edges containing $u$.
			\STATE Sort the $\{v\}_{i=1}^K$ in the descending order of $(u, v_i)$'s weight.
			\FOR {$i=1, \dots, \min(5, K)$}
				\IF{edge $(u, v_i)$ not in $\mathcal{G}$}
					\STATE Add undirected edge $(u, v_i)$ to $\mathcal{G}$.
				\ENDIF
			\ENDFOR

		\ENDFOR
	\ENDFOR
\ENSURE Undirected graph $\mathcal{G}$.
\end{algorithmic}
\end{algorithm}

\textbf{\textit{Architecture of Deep Models}}. We set the backbone of the user-preference model as a three-layer plain-DNN, each layer of which has 128, 64 and 24 hidden units respectively with PReLU \cite{xu2015empirical} activation function. As for ConTDM, the graph convolutional layer (two layers with hidden units of 72 and 24) is placed prior to the backbone and the parent fusion layer (a layer with hidden units of 24) is inserted right after the last layer of the backbone.

\textbf{\textit{Hyper-parameters for Training}}. For all those deep models, we set initial learning rate as $10^{-3}$ and decay learning rate by 0.9 every 100,000 iterations (UserBehavior) / 20,000 iterations (Amazon Books). We train these models with the batch size of 30,000 (UserBehavior) / 20,000 (Amazon Books) till they converge. Specifically, we train JTM and ConTDM with 4 (UserBehavior) / 15 (Amazon Books) epochs.

\textbf{\textit{Hyper-parameters for Prediction}}. For all the tree-based methods, we start predict from the $9^{th}$ level and send all those nodes (512 nodes) to the deep model for the first round prediction. We then pick the top 200 nodes in the descending order of their predicted scores as the recalled candidates of the current level. Next, children of those 200 picked nodes (i.e., 400 children) will be processed for the next round. We repeat these operations level by level till 200 leaf nodes are generated as the final retrieval set. But for all those methods with the multipath tree, owing to the efficiency provided by multipath parent fusion layer, we double the quota, i.e., 400 nodes, for retrieval in each level except the leaf level. Besides, with its multipath structure, we send both the graph-children and original children to predict for the next level.

% GE, MTL
%ConTDM and its variants process two sets of nodes at the same time, i.e. original samples from the tree index and their corresponding parent nodes. Before going through the backbone layers, each of them is processed by the Graph Embedding Unit(two-layer plain-DNN with hidden units of 72 and 24). Once obtained the features yielded by backbone layers, the Attention Unit(a single-layer plain-DNN with width of 24) takes those features from two sets as inputs and produces the fusion feature. While ConTDM directly apply SoftMax to the fusion feature, ConTDM-4k along with ConTDM-Multipath further blend the fusion feature with the embeddings of the next layers' candidates before the classification layer. By default, ConTDM and ConTDM-4k follows JTM to use the hierarchical user preference representation which cannot be directly applied to ConTDM-Multipath due to the multiple trace up choices. Therefore, we build a heuristic method of item trace up for ConTDM-Multipath: given the selected path of the well-trained ConTDM-4k model, for every leaf item, we count the most frequent node layer by layer which co-occurs with the leaf-item in all paths; meanwhile, the chosen nodes hold the graph parent-child linkage and finally form a trace up path to the root for the current leaf item. 

% ConTDM use the fixed well-trained JTM tree
%As for tree learning, we follow the procedures proposed in the paper \cite{zhu2019joint} to train the tree iteratively for JTM baseline. ConTDM and its variants directly use the well-trained tree from JTM and fix the tree during the whole process.

\section{Effectiveness Analysis of multipath Tree and parent fusion layer} \label{appendix:effectiveness}

In order to prove that our method is applicable in most cases, we carry out further experiments based on different trees and network structures. To exclude the influence brought by graph convolutional layer, we verify the validity of parent fusion layer on top of the aforementioned three-layer plain-DNN. Besides, since JTM tree requires time-consuming iterative tree learning, we additionally use other kinds of ordinary tree structures to validate the effectiveness of the multipath transformation. Specifically, we follow the settings of TDM\cite{zhu2018learning}, i.e.,  category-based initialized tree (denoted by \texttt{cate tree}) and completely random initialized tree (denoted by \texttt{rand tree}) for UserBehavior and Amazon Books respectively.

\begin{table*}[htbp]
	\caption{Ablation results for parent fusion layer and multipath Tree Index in Amazon Books and UserBehavior.} % add baseline and methods under dashline
	\label{table:AblationResultsPFMT}
\begin{tabular}{cccccccccccc}
\hlineB{2}
\multirow{2}{*}{Dataset} & \multirow{2}{*}{Tree Index} & \multirow{2}{*}{Model} & \multicolumn{3}{c}{Baseline}      & \multicolumn{3}{c}{4k}        & \multicolumn{3}{c}{multipath}                        \\ \cline{4-12}
                         &                             &                             & Precision & Recall  & F-score & Precision & Recall  & F-score & Precision       & Recall           & F-score         \\ \hlineB{2}
\multirow{4}{*}{UserBehavior}      & \multirow{2}{*}{JTM tree}   & DNN                         & 2.95\%    & 13.97\% & 4.44\%  & 2.91\%    & 13.85\% & 4.39\%  & \textbf{3.02\%} & \textbf{14.30\%} & \textbf{4.54\%} \\
                         &                             & DNN-PF                     & 3.09\%    & 14.66\% & 4.66\%  & 3.13\%    & 14.84\% & 4.71\%  & \textbf{3.15\%} & \textbf{14.97\%} & \textbf{4.76\%} \\ \cline{2-12} 
                         & \multirow{2}{*}{cate tree}  & DNN                         & 2.61\%    & 12.62\% & 3.95\%  & 2.69\%    & 12.95\% & 4.07\%  & \textbf{2.86\%} & \textbf{13.65\%} & \textbf{4.32\%} \\
                         &                             & DNN-PF                     & 2.73\%    & 13.26\% & 4.14\%  & 2.88\%    & 13.79\% & 4.35\%  & \textbf{3.05\%} & \textbf{14.41\%} & \textbf{4.59\%} \\ \hline
\multirow{4}{*}{Amazon Books}      & \multirow{2}{*}{JTM tree}   & DNN                         & 0.75\%    & 12.07\% & 1.34\%  & 0.75\%    & 12.02\% & 1.33\%  & \textbf{0.78\%} & \textbf{12.58\%} & \textbf{1.38\%} \\
                         &                             & DNN-PF                     & 0.76\%    & 12.31\% & 1.36\%  & 0.76\%    & 12.38\% & 1.36\%  & \textbf{0.78\%} & \textbf{12.78\%} & \textbf{1.39\%} \\ \cline{2-12} 
                         & \multirow{2}{*}{rand tree}  & DNN                         & 0.69\%    & 10.83\% & 1.22\%  & 0.69\%    & 10.91\% & 1.23\%  & \textbf{0.78\%} & \textbf{12.54\%} & \textbf{1.39\%} \\
                         &                             & DNN-PF                     & 0.71\%    & 11.13\% & 1.25\%  & 0.74\%    & 11.74\% & 1.31\%  & \textbf{0.79\%} & \textbf{13.16\%} & \textbf{1.41\%} \\ \hlineB{2}
\end{tabular}
\end{table*}

As is shown in Table \ref{table:AblationResultsPFMT}, both parent fusion layer and multipath tree lead to the improvements on all metrics. The recall lift brought by parent fusion layer are 2\%\textasciitilde5\% and 5\%\textasciitilde7\% in Amazon Books and UserBehaviors separately. However, multipath tree performs better in Amazon Books than in Userbehavior. \textbf{These two phenomena are consistent with the results of using ConTDM, which further illustrates that the difference of the tree index is responsible for this situation}.

In both datasets, multipath tree achieves more increase by using cate/rand tree than that of JTM tree. Specifically, with rand tree, multipath tree gains recall improvements by over 15\% while the lift gain with JTM tree is about 3\%\textasciitilde4\%. However, it is worth mentioning that the highest recall comes to the combination of parent fusion layer, multipath tree and rand tree, which is the only version that the non-JTM tree beats JTM tree using the same model. \textbf{It is proved again that multipath tree helps find a better graph-parent node and the parent fusion layer can finally lift the recall.}

Note that the current version of multipath tree relies on the graph built beforehand. \textbf{The multipath paradigm can be easily adapted to any other kinds of node relationships, which can potentially achieve even greater progress with appropriate prior knowledge.}

\begin{table}[!htbp]
\small
	\caption{Computation Cost Analysis between ConTDM and ConTDM-Multipath} % add baseline and methods under dashline
	\label{table:ComputationCost}
\begin{tabular}{r|ccc}
\hlineB{2}
Component         & \multicolumn{3}{c}{Computation Cost}                 \\ \hline
GC Layer          & (144*72+72*24)*11 &        &                         \\
Layer1            & 264*128           &        &                         \\
Layer2            & 128*64            &        &                         \\
Layer3            & 64*24             &        &                         \\
Softmax Layer            & 24*2              &        &                         \\ \hline
+PF Layer         &                   & +72*24 &                         \\
+Multipath   &                   &        & +72*24*(k+2)+24*2*k \\ \hline
Total             & 176624            & 178352 & 190688 (avg\_k=5)                  \\
Increase & +0\%              & +1.0\% & +8.0\%                 \\ \hlineB{2}
\end{tabular}
\end{table}

\section{Computation Cost Analysis}\label{appendix:computation}
ConTDM-Multipath can achieve a huge improvement while maintaining a small increase in computing costs during prediction. Table \ref{table:ComputationCost} illustrates the computation cost (FLOPs of prediction per sample) of ConTDM-Multipath over ConTDM.

We overlook the cost brought by bias calculation which is dispensable when compared to the time-consuming multiplication operations. Note that layers numbered from Layer1 to Layer3 compose the aforementioned DNN backbone where samples are processed with the shape of \texttt{(batch\_size, hidden\_dim)}. While the graph convolutional layer deals with grouped raw input which is in the shape of \texttt{(batch\_size, group\_len, embed\_dim)}, we take the \texttt{group\_len} into consideration as the last two dimensions of the tensor will be squashed as one afterwards. In our implementation, the \texttt{group\_len} is set to 11. As for multipath tree, the graph-children as well as the original children from the tree index serve as the target nodes for the coming level. We count the average graph-children number of each level. Since the average number ranges from 3 to 6, we empirically choose the average graph-children number (denote by k in the Table \ref{table:ComputationCost}) as 5 for comparison.

According to the level-wise beam search, the parent of the current node is processed beforehand. Therefore, we keep the candidates' Layer3 feature in the memory and reuse them in the parent fusion layer for the next level. Similarly, as for the multipath tree, children nodes sharing the same ancestor path hold exactly one copy of the parent feature.

It is clearly shown that parent fusion layer has little effect to the total amount of calculation. Only when proceeding in multipath tree with the doubled quota, the total cost rises by 8.0\%, which is acceptable considering the corresponding recall lift.

%	GE：(144*72+72*24)*11
%	Layer1：264*128
%	Layer2：128*64
%	Layer3：64*24
%	Layer4：24*2    →               +72*24     →    +2*(72*24*(k+2)+24*2*k)，max_k=6，avg_k=5
%FLOPS         176624            178352(+1.0%)            avg_k=5，203024(+13.8%)

%Tree: Category Tree or JTM
%BaseModel: AttDnn
%Metric: Precision, recall, F-measure
%There should be a big table Compare the best results of ConTDM(maybe include results on multi-way tree) with baseline methods on each dataset above
%Baseline method Youtube-Dnn,HSM(Hierarchical soft-max),JTM
